# Supplementary material for: Questioning the Coverage-Length Metric in Conformal Prediction: When Shorter Intervals Are Not Better
Source: arXiv:2601.21455 source file (2026-06-16)
Supplement: Supplementary file 1 [file supplements.tex]

\begin{table}[t]
\caption{Comparison between VCP and PCP under different $\alpha$ levels.}
\label{tab:motivating_example}
\begin{center}
\begin{small}
\begin{tabular}{lcccccc}
\toprule
$\alpha$ & $p$ & \multicolumn{2}{c}{VCP} & \multicolumn{2}{c}{PCP} \\
\cmidrule(lr){3-4} \cmidrule(lr){5-6}
         &     & Coverage & Length & Coverage & Length \\
\midrule
\multirow{3}{*}{0.10} 
  & 0.96 & 0.906 \scriptsize{$\pm 0.008$} & 22.894 \scriptsize{$\pm 0.308$} & 0.909 \scriptsize{$\pm 0.012$} & 22.614 \scriptsize{$\pm 0.568$} \\
  & 0.98 & 0.906 \scriptsize{$\pm 0.008$} & 22.894 \scriptsize{$\pm 0.308$} & 0.904 \scriptsize{$\pm 0.010$} & 22.714 \scriptsize{$\pm 0.369$} \\
  & 1    & 0.906 \scriptsize{$\pm 0.008$} & 22.894 \scriptsize{$\pm 0.308$} & 0.906 \scriptsize{$\pm 0.008$} & 22.894 \scriptsize{$\pm 0.308$} \\
\midrule
\multirow{3}{*}{0.20} 
  & 0.96 & 0.792 \scriptsize{$\pm 0.024$} & 21.886 \scriptsize{$\pm 0.279$} & 0.799 \scriptsize{$\pm 0.025$} & 21.255 \scriptsize{$\pm 0.303$} \\
  & 0.98 & 0.792 \scriptsize{$\pm 0.024$} & 21.886 \scriptsize{$\pm 0.279$} & 0.796 \scriptsize{$\pm 0.023$} & 21.589 \scriptsize{$\pm 0.334$} \\
  & 1    & 0.792 \scriptsize{$\pm 0.024$} & 21.886 \scriptsize{$\pm 0.279$} & 0.792 \scriptsize{$\pm 0.024$} & 21.886 \scriptsize{$\pm 0.279$} \\
\bottomrule
\end{tabular}
\end{small}
\end{center}
\vspace{-1em}
\end{table}
